# Supplementary material for: Can Model Compression Improve NLP Fairness
Source: arXiv:2201.08542 source file (2022-01-21)
Supplement: Supplementary file 1 [file appendix.tex]

\label{sec:appendix}
This is an appendix.
